# Supplementary material for: First Measurement of Differential Charged Current Quasielastic-like $\nu_\mu$-Argon Scattering Cross Sections with the MicroBooNE Detector
Source: arXiv:2006.00108 ancillary file (2020-10-06)
Supplement: Supplementary file 1 [file Supp_arXiv.pdf]

**Supplemental Materials: First measurement of differential charged current  
quasielastic-like  $\nu_\mu$ -argon scattering cross-sections using the MicroBooNE detector**  
(Dated: September 8, 2020)

**CROSS SECTION VALUES**

Tables I–IV include the single differential cross sections as a function of muon and proton kinematics for  $-0.65 < \cos(\theta_\mu) < 0.95$ , while the relevant results can be located in `CrossSectionsFullPhaseSpace.txt`. Tables VII–X show the same results for  $-0.65 < \cos(\theta_\mu) < 0.8$ , while the relevant values can be located in `CrossSectionsLimitedPhaseSpace.txt`.

TABLE I: Differential charged current quasielastic-like  $\nu_\mu$ - $^{40}\text{Ar}$  scattering cross-sections as a function of the muon scattering angle for  $-0.65 < \cos(\theta_\mu) < 0.95$ .

| Bin Number                                                                  | $\cos\theta_\mu$ Range | $d\sigma/d\cos\theta_\mu$<br>[ $10^{-38} \text{ cm}^2$ ] | Total Uncertainty<br>[ $10^{-38} \text{ cm}^2$ ] | Efficiency |
|-----------------------------------------------------------------------------|------------------------|----------------------------------------------------------|--------------------------------------------------|------------|
| 1                                                                           | [ -0.65 , -0.41 )      | -0.04                                                    | 0.47                                             | 0.13       |
| 2                                                                           | [ -0.41 , -0.17 )      | 2.72                                                     | 1.2                                              | 0.13       |
| 3                                                                           | [ -0.17 , 0.07 )       | 1.07                                                     | 0.61                                             | 0.15       |
| 4                                                                           | [ 0.07 , 0.32 )        | 2.54                                                     | 0.76                                             | 0.19       |
| 5                                                                           | [ 0.32 , 0.56 )        | 3.25                                                     | 1.12                                             | 0.21       |
| 6                                                                           | [ 0.56 , 0.80 )        | 7.23                                                     | 1.83                                             | 0.21       |
| 7                                                                           | [ 0.80 , 0.95 )        | 5.85                                                     | 1.85                                             | 0.21       |
| Total Integrated Cross Section [ $10^{-38} \text{ cm}^2$ ]: $4.93 \pm 1.55$ |                        |                                                          |                                                  |            |

TABLE II: Differential charged current quasielastic-like  $\nu_\mu$ - $^{40}\text{Ar}$  scattering cross-sections as a function of the muon momentum for  $-0.65 < \cos(\theta_\mu) < 0.95$ .

| Bin Number                                                                  | $P_\mu$ Range   | $d\sigma/dP_\mu$<br>[ $10^{-38} \text{ cm}^2/(\text{GeV}/c)$ ] | Total Uncertainty<br>[ $10^{-38} \text{ cm}^2/(\text{GeV}/c)$ ] | Efficiency |
|-----------------------------------------------------------------------------|-----------------|----------------------------------------------------------------|-----------------------------------------------------------------|------------|
| 1                                                                           | [ 0.10 , 0.30 ) | 1.95                                                           | 1.24                                                            | 0.16       |
| 2                                                                           | [ 0.30 , 0.50 ) | 8.91                                                           | 2.03                                                            | 0.22       |
| 3                                                                           | [ 0.50 , 0.70 ) | 7.23                                                           | 1.69                                                            | 0.22       |
| 4                                                                           | [ 0.70 , 0.90 ) | 3.29                                                           | 1.04                                                            | 0.2        |
| 5                                                                           | [ 0.90 , 1.10 ) | 1.78                                                           | 1.05                                                            | 0.17       |
| 6                                                                           | [ 1.10 , 1.30 ) | 0.94                                                           | 0.51                                                            | 0.16       |
| 7                                                                           | [ 1.30 , 1.50 ) | 0.54                                                           | 0.51                                                            | 0.17       |
| Total Integrated Cross Section [ $10^{-38} \text{ cm}^2$ ]: $4.93 \pm 1.55$ |                 |                                                                |                                                                 |            |

TABLE III: Differential charged current quasielastic-like  $\nu_\mu$ - $^{40}\text{Ar}$  scattering cross-sections as a function of the proton scattering angle for  $-0.65 < \cos(\theta_\mu) < 0.95$ .

| Bin Number                                                                  | $\cos\theta_p$ Range | $d\sigma/d\cos\theta_p$<br>[ $10^{-38} \text{ cm}^2$ ] | Total Uncertainty<br>[ $10^{-38} \text{ cm}^2$ ] | Efficiency |
|-----------------------------------------------------------------------------|----------------------|--------------------------------------------------------|--------------------------------------------------|------------|
| 1                                                                           | [ 0.15 , 0.26 )      | 3.11                                                   | 1.7                                              | 0.13       |
| 2                                                                           | [ 0.26 , 0.37 )      | 4.18                                                   | 1.9                                              | 0.23       |
| 3                                                                           | [ 0.37 , 0.47 )      | 3.2                                                    | 1.37                                             | 0.21       |
| 4                                                                           | [ 0.47 , 0.58 )      | 4.8                                                    | 1.75                                             | 0.22       |
| 5                                                                           | [ 0.58 , 0.69 )      | 9.36                                                   | 2.28                                             | 0.21       |
| 6                                                                           | [ 0.69 , 0.80 )      | 7.99                                                   | 2.32                                             | 0.2        |
| 7                                                                           | [ 0.80 , 0.95 )      | 6.72                                                   | 2.21                                             | 0.18       |
| Total Integrated Cross Section [ $10^{-38} \text{ cm}^2$ ]: $4.93 \pm 1.55$ |                      |                                                        |                                                  |            |

TABLE IV: Differential charged current quasielastic-like  $\nu_\mu$ - $^{40}\text{Ar}$  scattering cross-sections as a function of the proton momentum for  $-0.65 < \cos(\theta_\mu) < 0.95$ .

| Bin Number                                                                  | $P_p$ Range     | $d\sigma/dP_p$<br>[ $10^{-38} \text{ cm}^2/(\text{GeV}/c)$ ] | Total Uncertainty<br>[ $10^{-38} \text{ cm}^2/(\text{GeV}/c)$ ] | Efficiency |
|-----------------------------------------------------------------------------|-----------------|--------------------------------------------------------------|-----------------------------------------------------------------|------------|
| 1                                                                           | [ 0.30 , 0.40 ) | 5.82                                                         | 3.15                                                            | 0.17       |
| 2                                                                           | [ 0.40 , 0.50 ) | 7.77                                                         | 3.31                                                            | 0.25       |
| 3                                                                           | [ 0.50 , 0.60 ) | 9.17                                                         | 2.95                                                            | 0.25       |
| 4                                                                           | [ 0.60 , 0.70 ) | 7.43                                                         | 2.52                                                            | 0.24       |
| 5                                                                           | [ 0.70 , 0.80 ) | 7.05                                                         | 1.94                                                            | 0.18       |
| 6                                                                           | [ 0.80 , 0.90 ) | 6.26                                                         | 2.29                                                            | 0.12       |
| 7                                                                           | [ 0.90 , 1.00 ) | 1.95                                                         | 1.69                                                            | 0.07       |
| Total Integrated Cross Section [ $10^{-38} \text{ cm}^2$ ]: $4.93 \pm 1.55$ |                 |                                                              |                                                                 |            |

TABLE V: Differential charged current quasielastic-like  $\nu_\mu$ - $^{40}\text{Ar}$  scattering cross-sections as a function of the reconstructed momentum transfer for  $-0.65 < \cos(\theta_\mu) < 0.95$ .

| Bin Number                                                                  | $Q_{CCQE}^2$ Range | $d\sigma/dQ_{CCQE}^2$<br>[ $10^{-38} \text{ cm}^2/(\text{GeV}/c)$ ] | Total Uncertainty<br>[ $10^{-38} \text{ cm}^2/(\text{GeV}^2/c^2)$ ] | Efficiency |
|-----------------------------------------------------------------------------|--------------------|---------------------------------------------------------------------|---------------------------------------------------------------------|------------|
| 1                                                                           | [ 0.00 , 0.17 )    | 2.92                                                                | 0.82                                                                | 0.27       |
| 2                                                                           | [ 0.17 , 0.34 )    | 9.92                                                                | 1.69                                                                | 0.21       |
| 3                                                                           | [ 0.34 , 0.51 )    | 8.64                                                                | 1.79                                                                | 0.17       |
| 4                                                                           | [ 0.51 , 0.69 )    | 4.51                                                                | 0.96                                                                | 0.15       |
| 5                                                                           | [ 0.69 , 0.86 )    | 1.69                                                                | 0.56                                                                | 0.13       |
| 6                                                                           | [ 0.86 , 1.03 )    | 0.9                                                                 | 0.33                                                                | 0.13       |
| 7                                                                           | [ 1.03 , 1.20 )    | 0.17                                                                | 0.13                                                                | 0.18       |
| Total Integrated Cross Section [ $10^{-38} \text{ cm}^2$ ]: $4.93 \pm 1.55$ |                    |                                                                     |                                                                     |            |

TABLE VI: Differential charged current quasielastic-like  $\nu_\mu$ - $^{40}\text{Ar}$  scattering cross-sections as a function of the reconstructed neutrino energy for  $-0.65 < \cos(\theta_\mu) < 0.95$ .

| Bin Number                                                                  | $E_\nu^{cal}$ Range | $d\sigma/dE_\nu^{cal}$<br>[ $10^{-38} \text{ cm}^2/(\text{GeV}/c)$ ] | Total Uncertainty<br>[ $10^{-38} \text{ cm}^2/(\text{GeV})$ ] | Efficiency |
|-----------------------------------------------------------------------------|---------------------|----------------------------------------------------------------------|---------------------------------------------------------------|------------|
| 1                                                                           | [ 0.30 , 0.47 )     | 1.74                                                                 | 0.51                                                          | 0.21       |
| 2                                                                           | [ 0.47 , 0.63 )     | 7.85                                                                 | 1.49                                                          | 0.26       |
| 3                                                                           | [ 0.63 , 0.80 )     | 6.13                                                                 | 1.18                                                          | 0.23       |
| 4                                                                           | [ 0.80 , 0.96 )     | 3.45                                                                 | 0.83                                                          | 0.2        |
| 5                                                                           | [ 0.96 , 1.13 )     | 1.44                                                                 | 0.55                                                          | 0.18       |
| 6                                                                           | [ 1.13 , 1.30 )     | 1.52                                                                 | 0.43                                                          | 0.15       |
| 7                                                                           | [ 1.30 , 1.46 )     | 0.88                                                                 | 0.29                                                          | 0.13       |
| Total Integrated Cross Section [ $10^{-38} \text{ cm}^2$ ]: $4.93 \pm 1.55$ |                     |                                                                      |                                                               |            |

TABLE VII: Differential charged current quasielastic-like  $\nu_\mu$ - $^{40}\text{Ar}$  scattering cross-sections as a function of the muon scattering angle for  $-0.65 < \cos(\theta_\mu) < 0.8$ .

| Bin Number                                                                  | $\cos\theta_\mu$ Range | $d\sigma/d\cos\theta_\mu$<br>[ $10^{-38} \text{ cm}^2$ ] | Total Uncertainty<br>[ $10^{-38} \text{ cm}^2$ ] | Efficiency |
|-----------------------------------------------------------------------------|------------------------|----------------------------------------------------------|--------------------------------------------------|------------|
| 1                                                                           | [ -0.65 , -0.41 )      | -0.04                                                    | 0.47                                             | 0.13       |
| 2                                                                           | [ -0.41 , -0.17 )      | 2.72                                                     | 1.2                                              | 0.13       |
| 3                                                                           | [ -0.17 , 0.07 )       | 1.07                                                     | 0.62                                             | 0.15       |
| 4                                                                           | [ 0.07 , 0.32 )        | 2.54                                                     | 0.75                                             | 0.19       |
| 5                                                                           | [ 0.32 , 0.56 )        | 3.25                                                     | 1.12                                             | 0.21       |
| 6                                                                           | [ 0.56 , 0.80 )        | 7.23                                                     | 1.83                                             | 0.21       |
| Total Integrated Cross Section [ $10^{-38} \text{ cm}^2$ ]: $4.05 \pm 1.40$ |                        |                                                          |                                                  |            |

TABLE VIII: Differential charged current quasielastic-like  $\nu_\mu$ - $^{40}\text{Ar}$  scattering cross-sections as a function of the muon momentum for  $-0.65 < \cos(\theta_\mu) < 0.8$ .

| Bin Number                                                                  | $P_\mu$ Range   | $d\sigma/dP_\mu$<br>[ $10^{-38} \text{ cm}^2/(\text{GeV}/c)$ ] | Total Uncertainty<br>[ $10^{-38} \text{ cm}^2/(\text{GeV}/c)$ ] | Efficiency |
|-----------------------------------------------------------------------------|-----------------|----------------------------------------------------------------|-----------------------------------------------------------------|------------|
| 1                                                                           | [ 0.10 , 0.30 ) | 2.01                                                           | 1.28                                                            | 0.16       |
| 2                                                                           | [ 0.30 , 0.50 ) | 8.73                                                           | 2.0                                                             | 0.22       |
| 3                                                                           | [ 0.50 , 0.70 ) | 6.32                                                           | 1.54                                                            | 0.2        |
| 4                                                                           | [ 0.70 , 0.90 ) | 2.27                                                           | 0.83                                                            | 0.17       |
| 5                                                                           | [ 0.90 , 1.10 ) | 0.87                                                           | 0.71                                                            | 0.17       |
| 6                                                                           | [ 1.10 , 1.30 ) | 0.07                                                           | 0.12                                                            | 0.22       |
| 7                                                                           | [ 1.30 , 1.50 ) | -0.01                                                          | 0.01                                                            | 0.29       |
| Total Integrated Cross Section [ $10^{-38} \text{ cm}^2$ ]: $4.05 \pm 1.40$ |                 |                                                                |                                                                 |            |

TABLE IX: Differential charged current quasielastic-like  $\nu_\mu$ - $^{40}\text{Ar}$  scattering cross-sections as a function of the proton scattering angle for  $-0.65 < \cos(\theta_\mu) < 0.8$ .

| Bin Number                                                                  | $\cos\theta_p$ Range | $d\sigma/d\cos\theta_p$<br>[ $10^{-38} \text{ cm}^2$ ] | Total Uncertainty<br>[ $10^{-38} \text{ cm}^2$ ] | Efficiency |
|-----------------------------------------------------------------------------|----------------------|--------------------------------------------------------|--------------------------------------------------|------------|
| 1                                                                           | [ 0.15 , 0.26 )      | 0.72                                                   | 0.51                                             | 0.13       |
| 2                                                                           | [ 0.26 , 0.37 )      | 3.3                                                    | 1.15                                             | 0.21       |
| 3                                                                           | [ 0.37 , 0.47 )      | 1.57                                                   | 0.76                                             | 0.26       |
| 4                                                                           | [ 0.47 , 0.58 )      | 3.69                                                   | 1.45                                             | 0.23       |
| 5                                                                           | [ 0.58 , 0.69 )      | 6.87                                                   | 1.74                                             | 0.2        |
| 6                                                                           | [ 0.69 , 0.80 )      | 7.83                                                   | 1.95                                             | 0.2        |
| 7                                                                           | [ 0.80 , 0.95 )      | 6.76                                                   | 2.12                                             | 0.18       |
| Total Integrated Cross Section [ $10^{-38} \text{ cm}^2$ ]: $4.05 \pm 1.40$ |                      |                                                        |                                                  |            |

TABLE X: Differential charged current quasielastic-like  $\nu_\mu$ - $^{40}\text{Ar}$  scattering cross-sections as a function of the proton momentum for  $-0.65 < \cos(\theta_\mu) < 0.8$ .

| Bin Number                                                                  | $P_p$ Range     | $d\sigma/dP_p$<br>[ $10^{-38} \text{ cm}^2/(\text{GeV}/c)$ ] | Total Uncertainty<br>[ $10^{-38} \text{ cm}^2/(\text{GeV}/c)$ ] | Efficiency |
|-----------------------------------------------------------------------------|-----------------|--------------------------------------------------------------|-----------------------------------------------------------------|------------|
| 1                                                                           | [ 0.30 , 0.40 ) | 4.71                                                         | 2.41                                                            | 0.17       |
| 2                                                                           | [ 0.40 , 0.50 ) | 3.89                                                         | 2.03                                                            | 0.25       |
| 3                                                                           | [ 0.50 , 0.60 ) | 7.93                                                         | 2.65                                                            | 0.25       |
| 4                                                                           | [ 0.60 , 0.70 ) | 6.4                                                          | 2.13                                                            | 0.25       |
| 5                                                                           | [ 0.70 , 0.80 ) | 5.16                                                         | 1.63                                                            | 0.18       |
| 6                                                                           | [ 0.80 , 0.90 ) | 5.75                                                         | 2.19                                                            | 0.11       |
| 7                                                                           | [ 0.90 , 1.00 ) | 2.27                                                         | 1.62                                                            | 0.07       |
| Total Integrated Cross Section [ $10^{-38} \text{ cm}^2$ ]: $4.05 \pm 1.40$ |                 |                                                              |                                                                 |            |

TABLE XI: Differential charged current quasielastic-like  $\nu_\mu$ - $^{40}\text{Ar}$  scattering cross-sections as a function of the reconstructed momentum transfer for  $-0.65 < \cos(\theta_\mu) < 0.8$ .

| Bin Number                                                                  | $Q_{CCQE}^2$ Range | $d\sigma/dQ_{CCQE}^2$<br>[ $10^{-38} \text{ cm}^2/(\text{GeV}/c)$ ] | Total Uncertainty<br>[ $10^{-38} \text{ cm}^2/(\text{GeV}^2/c^2)$ ] | Efficiency |
|-----------------------------------------------------------------------------|--------------------|---------------------------------------------------------------------|---------------------------------------------------------------------|------------|
| 1                                                                           | [ 0.00 , 0.17 )    | 1.41                                                                | 0.52                                                                | 0.26       |
| 2                                                                           | [ 0.17 , 0.34 )    | 7.54                                                                | 1.37                                                                | 0.23       |
| 3                                                                           | [ 0.34 , 0.51 )    | 7.76                                                                | 1.64                                                                | 0.18       |
| 4                                                                           | [ 0.51 , 0.69 )    | 4.07                                                                | 0.9                                                                 | 0.15       |
| 5                                                                           | [ 0.69 , 0.86 )    | 1.7                                                                 | 0.56                                                                | 0.12       |
| 6                                                                           | [ 0.86 , 1.03 )    | 0.93                                                                | 0.33                                                                | 0.13       |
| 7                                                                           | [ 1.03 , 1.20 )    | 0.17                                                                | 0.13                                                                | 0.18       |
| Total Integrated Cross Section [ $10^{-38} \text{ cm}^2$ ]: $4.05 \pm 1.40$ |                    |                                                                     |                                                                     |            |

TABLE XII: Differential charged current quasielastic-like  $\nu_\mu$ - $^{40}\text{Ar}$  scattering cross-sections as a function of the reconstructed neutrino energy for  $-0.65 < \cos(\theta_\mu) < 0.8$ .

| Bin Number                                                                  | $E_\nu^{cal}$ Range | $d\sigma/dE_\nu^{cal}$<br>[ $10^{-38} \text{ cm}^2/(\text{GeV}/c)$ ] | Total Uncertainty<br>[ $10^{-38} \text{ cm}^2/(\text{GeV})$ ] | Efficiency |
|-----------------------------------------------------------------------------|---------------------|----------------------------------------------------------------------|---------------------------------------------------------------|------------|
| 1                                                                           | [ 0.30 , 0.47 )     | 1.85                                                                 | 0.53                                                          | 0.21       |
| 2                                                                           | [ 0.47 , 0.63 )     | 8.25                                                                 | 1.53                                                          | 0.25       |
| 3                                                                           | [ 0.63 , 0.80 )     | 5.42                                                                 | 1.05                                                          | 0.22       |
| 4                                                                           | [ 0.80 , 0.96 )     | 2.05                                                                 | 0.64                                                          | 0.18       |
| 5                                                                           | [ 0.96 , 1.13 )     | 0.65                                                                 | 0.31                                                          | 0.14       |
| 6                                                                           | [ 1.13 , 1.30 )     | 0.6                                                                  | 0.26                                                          | 0.12       |
| 7                                                                           | [ 1.30 , 1.46 )     | 0.08                                                                 | 0.11                                                          | 0.12       |
| Total Integrated Cross Section [ $10^{-38} \text{ cm}^2$ ]: $4.05 \pm 1.40$ |                     |                                                                      |                                                               |            |

## COVARIANCE MATRICES

Figure 1 shows the total covariance matrices, which include both statistical and systematic uncertainties for events in the full available phase-space with  $-0.65 < \cos(\theta_\mu) < 0.95$ , while the relevant entries are provided in `microbooneCCQECovarianceMatrixFullPhaseSpace.txt`.

Fig 2 shows the same results in the limited available phase-space with  $-0.65 < \cos(\theta_\mu) < 0.8$ , while the relevant entries are provided in `microbooneCCQECovarianceMatrixLimitedPhaseSpace.txt`.

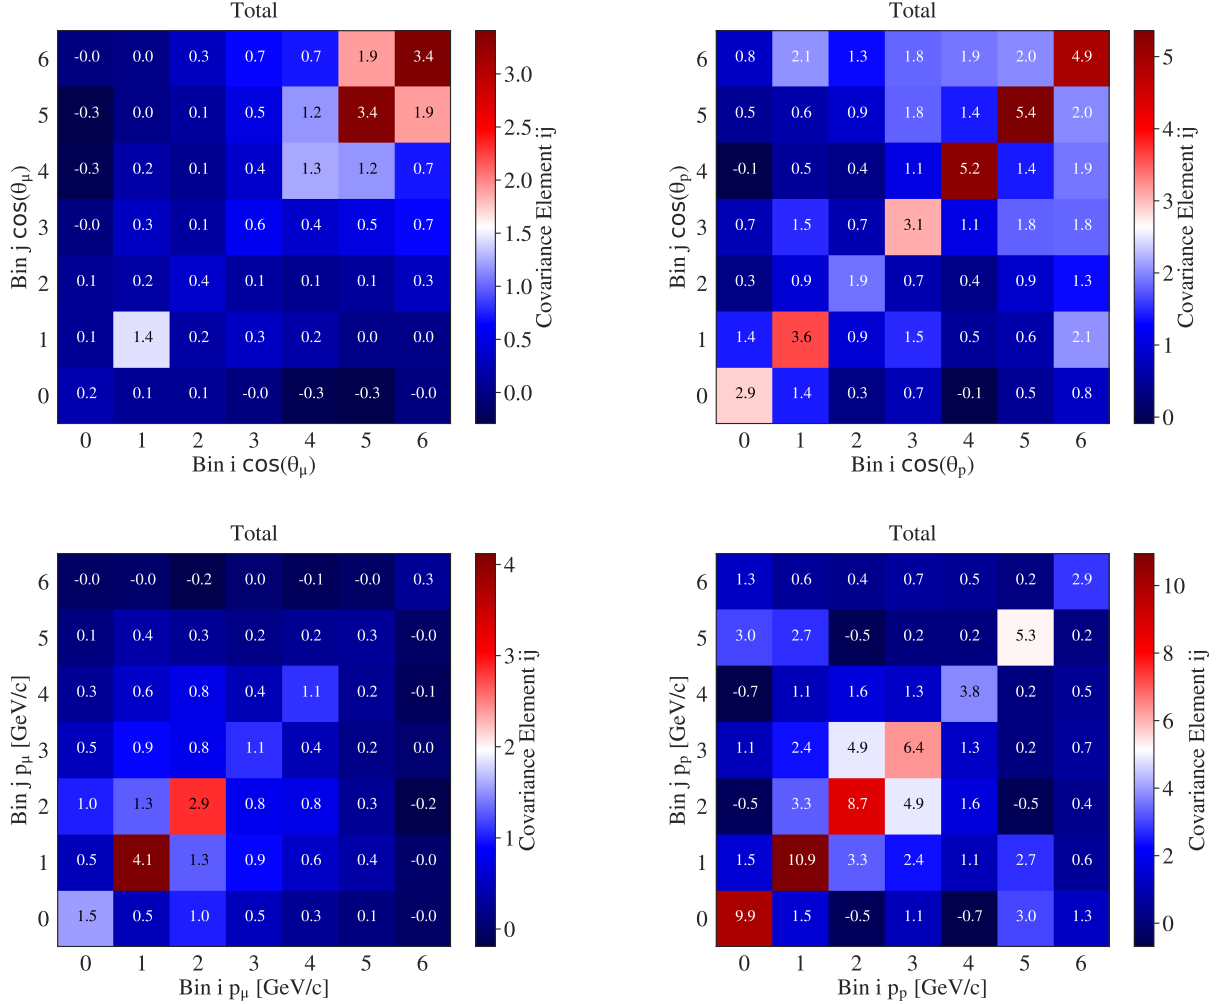

FIG. 1. Total covariance matrix for the muon and proton scattering angle and momentum for events with  $-0.65 < \cos(\theta_\mu) < 0.95$ .

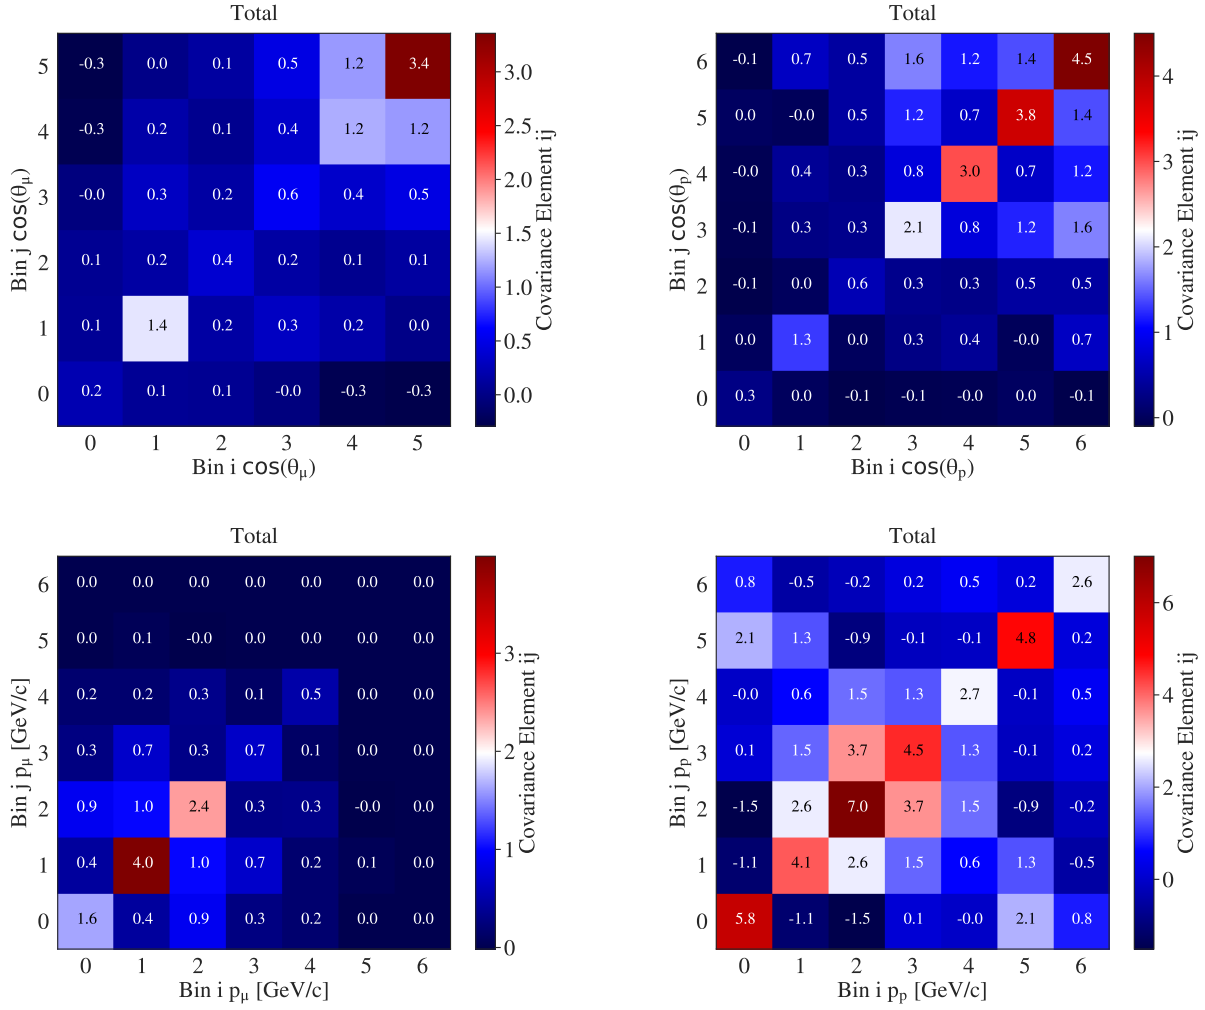

FIG. 2. Total covariance matrix for the muon and proton scattering angle and momentum for events with  $-0.65 < \cos(\theta_\mu) < 0.8$ .

## SMEARING MATRICES

The smearing matrix  $S$  transforms the number of generated events in bin  $i$  of generated momentum or scattering angle,  $N_{\text{gen}}^i$  to the number of events in bin  $j$  of measured momentum or scattering angle,  $N_{\text{reco}}^j$ . Figure 3 shows the smearing matrices for the muon and proton scattering angle and momentum in order for the reader to assess the size of the bin migration corrections we apply to the data. The values of the smearing matrix are provided in the attached text file `microbooneCCQESmearingMatrix.txt`.

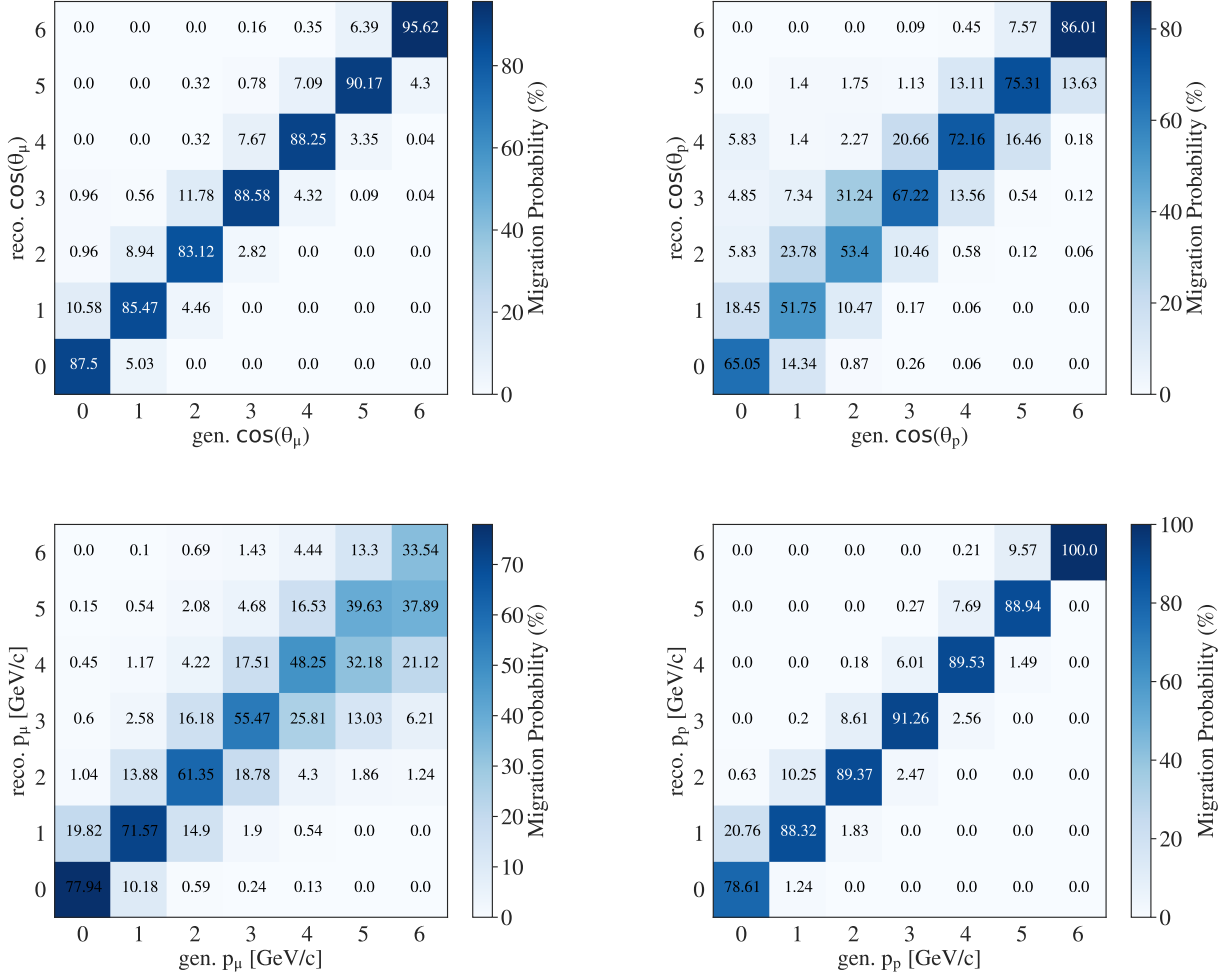

FIG. 3. Smearing matrices. The top (bottom) plot shows the scattering angle (momentum) smearing matrices for the muon and the proton.

## HIGH-LEVEL VARIABLES AND KINEMATIC CORRELATIONS

The smearing matrices for the complex variables  $Q_{CCQE}^2 = (E_\nu^{cal} - E_\mu)^2 - (\vec{p}_\nu - \vec{p}_\mu)^2$  and  $E_\nu^{cal} = E_\mu + T_p + BE$  are shown in figure 4, while figure 5 shows the correlation between  $Q_{CCQE}^2$  and  $\cos(\theta_\mu)$ , where the black vertical lines indicate the limits of the last  $\cos(\theta_\mu)$  bin.

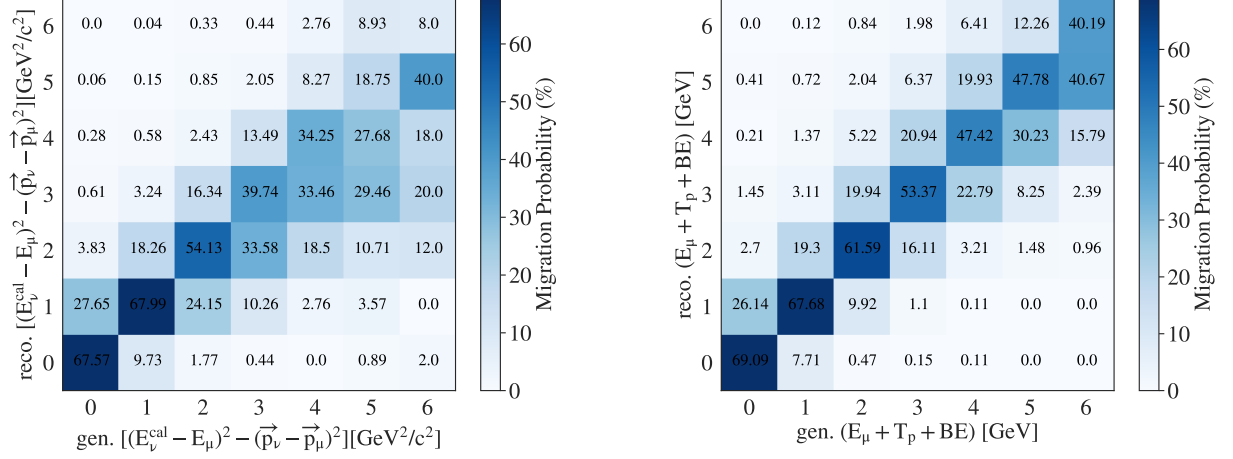

FIG. 4. Smearing matrices for the high-level variables  $Q_{CCQE}^2 = (E_\nu^{cal} - E_\mu)^2 - (\vec{p}_\nu - \vec{p}_\mu)^2$  (left) and  $E_\nu^{cal} = E_\mu + T_p + BE$  (right).

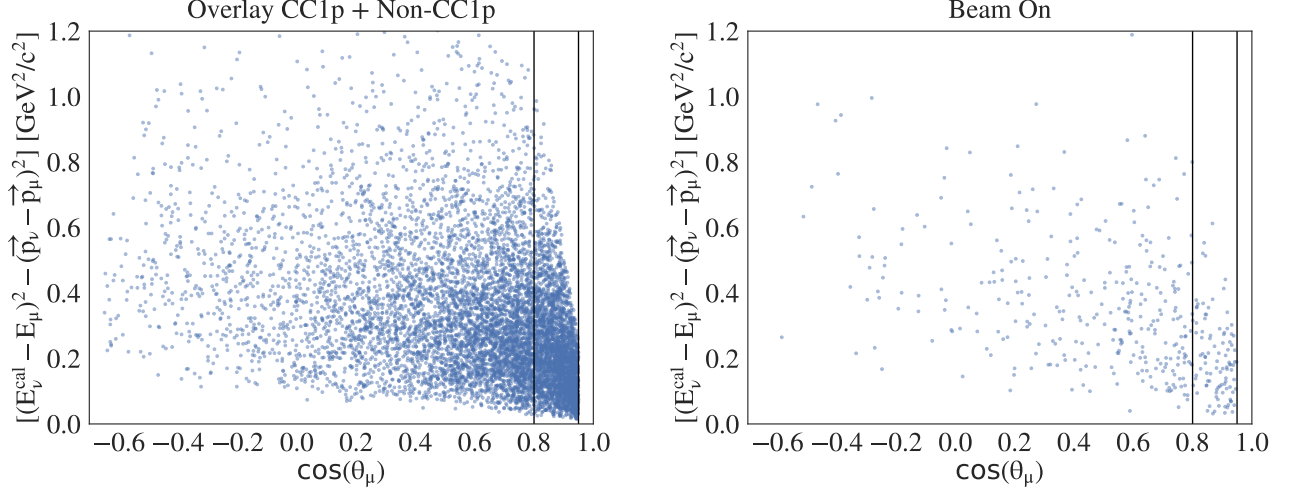

FIG. 5. Kinematic correlations between the high-level variable  $Q_{CCQE}^2 = (E_\nu^{cal} - E_\mu)^2 - (\vec{p}_\nu - \vec{p}_\mu)^2$  and  $\cos(\theta_\mu)$  for the overlay sample (left) and beam on (right). The black vertical lines indicate the limits of the last  $\cos(\theta_\mu)$  bin.

## SIMULATED BEAM RELATED BACKGROUND

This section details all contributions to the simulated beam related background passing the analysis event selection. Table XIII details the fractional contribution of non  $\mu - p$  pairs, and  $\mu - p$  pairs not CC1p0 $\pi$  using truth level information, for example events with a muon, proton and an additional proton or pions left undetected due to detector inefficiencies. Table XIV details the contribution of the different other pairs (non  $\mu - p$  pairs), while Tables XV– XVIII show the number of events for the data, the cosmic background, the CC1p signal, the beam related MC background and the fraction of the latter over the CC1p signal as a function of the kinematic variables of interest, after normalizing to  $4.59 \times 10^{19}$  POT. Figures 6–8 illustrate this non-negligible contribution originating from beam related MC background events.

TABLE XIII: The number of simulated beam related background events from different sources passing the analysis event selection cuts. The “beam-on” equivalent column lists the number of events scaled to the beam-on available POT.

| background pairs                | number of events | beam-on equivalent | fractional contribution to beam-on |
|---------------------------------|------------------|--------------------|------------------------------------|
| $\mu - p$ pairs not CC1p0 $\pi$ | $1204 \pm 34.7$  | $82.6 \pm 2.4$     | $20.2 \pm 1.3\%$                   |
| other non $\mu - p$ pairs       | $172 \pm 13.1$   | $11.8 \pm 0.9$     | $2.9 \pm 0.4\%$                    |

TABLE XIV: The number of simulated beam related background events from the other non  $\mu - p$  pairs passing the analysis event selection cuts. The “beam-on” equivalent column lists the number of events scaled to the beam-on available POT.

| background pairs | number of events | beam-on equivalent | fractional contribution to beam-on |
|------------------|------------------|--------------------|------------------------------------|
| broken tracks    | $13 \pm 3.6$     | $0.9 \pm 0.2$      | $0.22 \pm 0.06\%$                  |
| $\mu^+ p$        | $11 \pm 3.3$     | $0.8 \pm 0.2$      | $0.18 \pm 0.06\%$                  |
| $pp$             | $18 \pm 4.2$     | $1.2 \pm 0.3$      | $0.30 \pm 0.07\%$                  |
| $\pi p$          | $109 \pm 10.4$   | $7.5 \pm 0.7$      | $1.82 \pm 0.20\%$                  |
| $ep$             | $19 \pm 4.4$     | $1.3 \pm 0.3$      | $0.32 \pm 0.07\%$                  |
| $\mu D$          | $1.0 \pm 1.0$    | $0.1 \pm 0.1$      | $0.02 \pm 0.02\%$                  |
| others           | $1.0 \pm 1.0$    | $0.1 \pm 0.1$      | $0.02 \pm 0.02\%$                  |

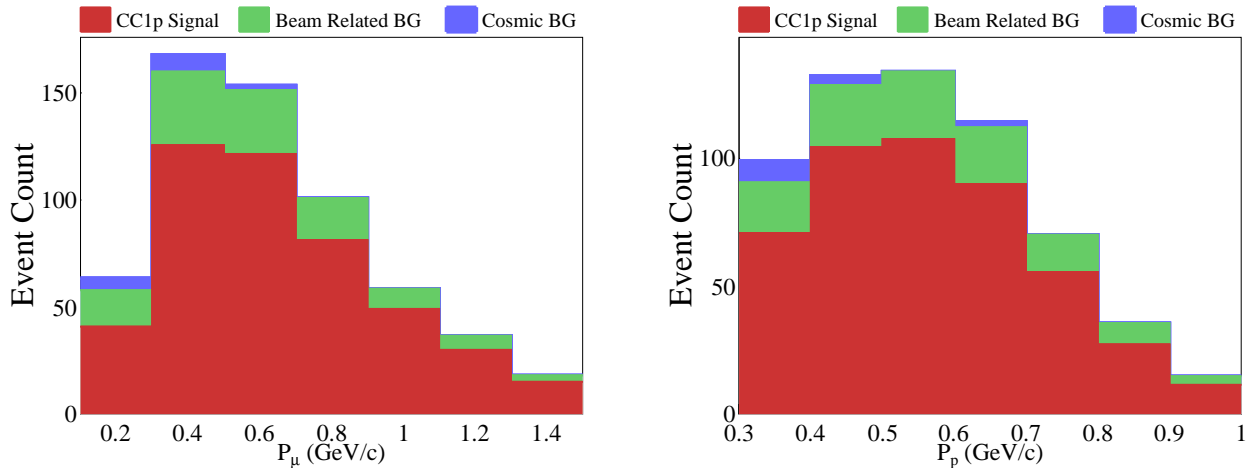

FIG. 6. The muon and proton momentum event distributions for the CC1p0 $\pi$  signal, the beam related background and the cosmic background.

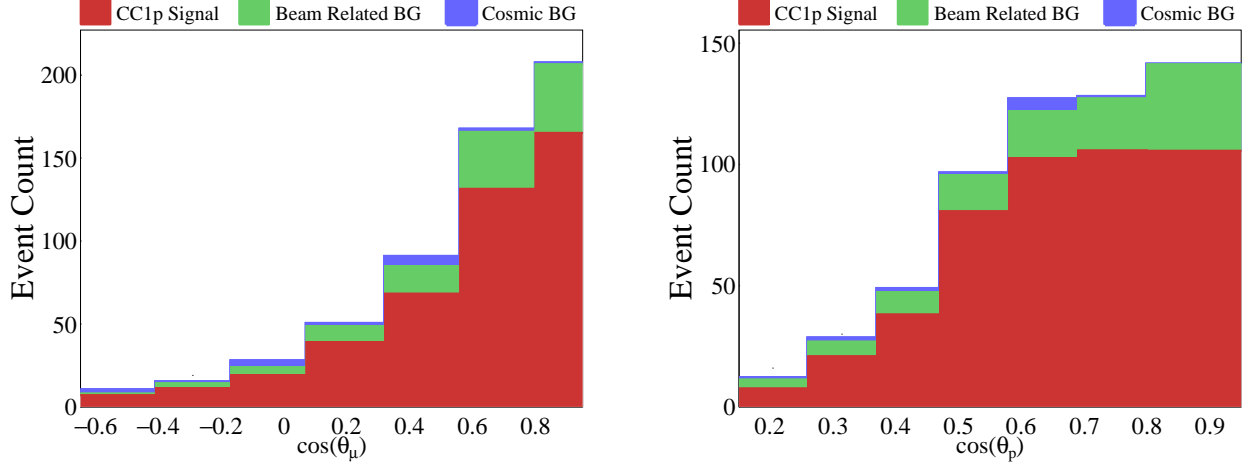

FIG. 7. The muon and proton angular event distributions for the CC1p0 $\pi$  signal, the beam related background and the cosmic background.

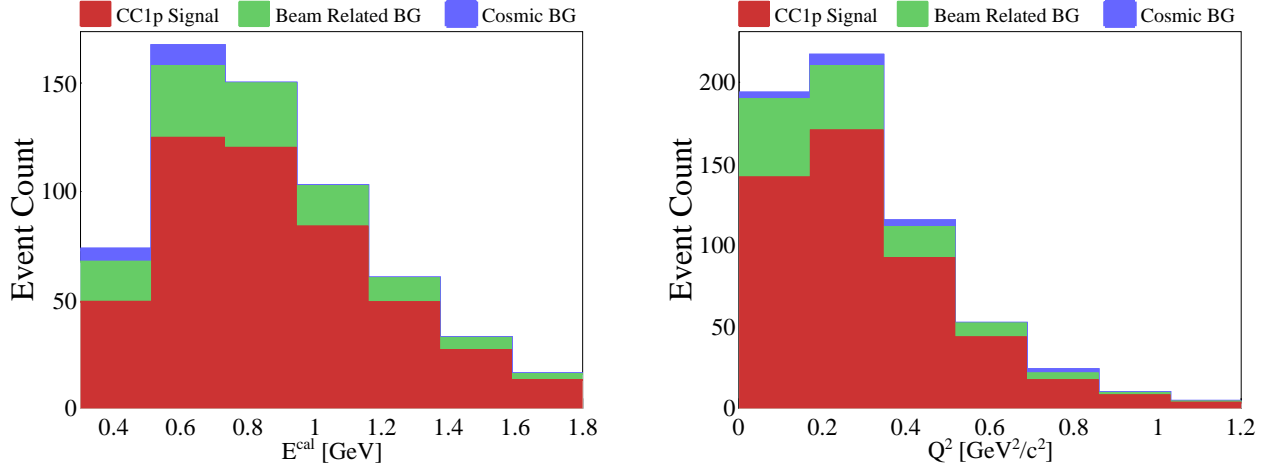

FIG. 8. The calorimetric energy reconstruction and 4-momentum transfer event distributions for the CC1p0 $\pi$  signal, the beam related background and the cosmic background.

TABLE XV: The number of events for the data, the cosmic background, the CC1p signal, the beam related MC background and the fraction of the latter over the CC1p signal as a function of  $\cos(\theta_\mu)$ , after normalizing to  $4.59 \times 10^{19}$  POT.

| $\cos(\theta_\mu)$<br>Bin Number | $\cos(\theta_\mu)$<br>Bin Range | Data | Cosmic<br>Background | CC1p<br>MC Signal | Beam Related<br>MC Background | $\frac{\text{Beam Related MC BG}}{\text{CC1p MC Signal}}$ (%) |
|----------------------------------|---------------------------------|------|----------------------|-------------------|-------------------------------|---------------------------------------------------------------|
| 1                                | [-0.65 , -0.41)                 | 5    | 2.12                 | 7.03              | 1.03                          | 14.6                                                          |
| 2                                | [-0.41 , -0.17)                 | 19   | 0.706                | 11.3              | 2.92                          | 25.8                                                          |
| 3                                | [-0.17 , 0.07)                  | 25   | 3.53                 | 19.2              | 4.92                          | 25.7                                                          |
| 4                                | [0.07 , 0.32)                   | 47   | 1.41                 | 39.1              | 9.64                          | 24.6                                                          |
| 5                                | [0.32 , 0.56)                   | 74   | 5.65                 | 68.3              | 16.7                          | 24.4                                                          |
| 6                                | [0.56 , 0.8)                    | 136  | 1.41                 | 131               | 34.4                          | 26.1                                                          |
| 7                                | [0.8 , 0.95)                    | 97   | 0.706                | 165               | 41.3                          | 25                                                            |

TABLE XVI: The number of events for the data, the cosmic background, the CC1p signal, the beam related MC background and the fraction of the latter over the CC1p signal as a function of  $\cos(\theta_p)$ , after normalizing to  $4.59 \times 10^{19}$  POT.

| $\cos(\theta_p)$<br>Bin Number | $\cos(\theta_p)$<br>Bin Range | Data | Cosmic<br>Background | CC1p<br>MC Signal | Beam Related<br>MC Background | $\frac{\text{Beam Related MC BG}}{\text{CC1p MC Signal}} (\%)$ |
|--------------------------------|-------------------------------|------|----------------------|-------------------|-------------------------------|----------------------------------------------------------------|
| 1                              | [0.15 , 0.26)                 | 16   | 0.706                | 7.59              | 3.69                          | 48.6                                                           |
| 2                              | [0.26 , 0.37)                 | 30   | 1.41                 | 20.9              | 6.05                          | 29                                                             |
| 3                              | [0.37 , 0.47)                 | 43   | 1.41                 | 38.1              | 9.23                          | 24.2                                                           |
| 4                              | [0.47 , 0.58)                 | 58   | 0.706                | 80.7              | 15                            | 18.6                                                           |
| 5                              | [0.58 , 0.69)                 | 77   | 4.94                 | 103               | 19.4                          | 18.9                                                           |
| 6                              | [0.69 , 0.8)                  | 78   | 0.706                | 106               | 21.5                          | 20.3                                                           |
| 7                              | [0.8 , 0.95)                  | 89   | 0                    | 106               | 35.6                          | 33.7                                                           |

TABLE XVII: The number of events for the data, the cosmic background, the CC1p signal, the beam related MC background and the fraction of the latter over the CC1p signal as a function of  $P_\mu$ , after normalizing to  $4.59 \times 10^{19}$  POT.

| $P_\mu$<br>Bin Number | $P_\mu$<br>Bin Range | Data | Cosmic<br>Background | CC1p<br>MC Signal | Beam Related<br>MC Background | $\frac{\text{Beam Related MC BG}}{\text{CC1p MC Signal}} (\%)$ |
|-----------------------|----------------------|------|----------------------|-------------------|-------------------------------|----------------------------------------------------------------|
| 1                     | [0.1 , 0.3)          | 40   | 5.65                 | 40.9              | 17                            | 41.5                                                           |
| 2                     | [0.3 , 0.5)          | 141  | 7.77                 | 126               | 34.4                          | 27.4                                                           |
| 3                     | [0.5 , 0.7)          | 121  | 2.12                 | 122               | 29.8                          | 24.5                                                           |
| 4                     | [0.7 , 0.9)          | 54   | 0                    | 81.3              | 19.6                          | 24.2                                                           |
| 5                     | [0.9 , 1.1)          | 31   | 0                    | 49.2              | 9.39                          | 19.1                                                           |
| 6                     | [1.1 , 1.3)          | 18   | 0                    | 30.1              | 6.56                          | 21.8                                                           |
| 7                     | [1.3 , 1.5)          | 9    | 0                    | 15.1              | 2.97                          | 19.7                                                           |

TABLE XVIII: The number of events for the data, the cosmic background, the CC1p signal, the beam related MC background and the fraction of the latter over the CC1p signal as a function of  $P_p$ , after normalizing to  $4.59 \times 10^{19}$  POT.

| $P_p$<br>Bin Number | $P_p$<br>Bin Range | Data | Cosmic<br>Background | CC1p<br>MC Signal | Beam Related<br>MC Background | $\frac{\text{Beam Related MC BG}}{\text{CC1p MC Signal}} (\%)$ |
|---------------------|--------------------|------|----------------------|-------------------|-------------------------------|----------------------------------------------------------------|
| 1                   | [0.3 , 0.4)        | 45   | 8.48                 | 70.9              | 19.7                          | 27.9                                                           |
| 2                   | [0.4 , 0.5)        | 90   | 3.53                 | 104               | 24.3                          | 23.3                                                           |
| 3                   | [0.5 , 0.6)        | 104  | 0                    | 108               | 26.4                          | 24.5                                                           |
| 4                   | [0.6 , 0.7)        | 67   | 2.12                 | 90                | 22.2                          | 24.7                                                           |
| 5                   | [0.7 , 0.8)        | 62   | 0                    | 55.6              | 14.5                          | 26.1                                                           |
| 6                   | [0.8 , 0.9)        | 33   | 0                    | 27.3              | 8.31                          | 30.5                                                           |
| 7                   | [0.9 , 1)          | 9    | 0                    | 11.5              | 3.33                          | 29                                                             |

TABLE XIX: The number of events for the data, the cosmic background, the CC1p signal, the beam related MC background and the fraction of the latter over the CC1p signal as a function of  $E^{cal}$ , after normalizing to  $4.59 \times 10^{19}$  POT.

| $E^{cal}$<br>Bin Number | $E^{cal}$<br>Bin Range | Data | Cosmic<br>Background | CC1p<br>MC Signal | Beam Related<br>MC Background | $\frac{\text{Beam Related MC BG}}{\text{CC1p MC Signal}} (\%)$ |
|-------------------------|------------------------|------|----------------------|-------------------|-------------------------------|----------------------------------------------------------------|
| 1                       | [0.3 , 0.514)          | 48   | 5.65                 | 49.2              | 18.5                          | 37.5                                                           |
| 2                       | [0.514 , 0.729)        | 132  | 9.18                 | 125               | 33.1                          | 26.6                                                           |
| 3                       | [0.729 , 0.943)        | 110  | 0                    | 120               | 29.6                          | 24.7                                                           |
| 4                       | [0.943 , 1.16)         | 70   | 0                    | 83.9              | 18.7                          | 22.3                                                           |
| 5                       | [1.16 , 1.37)          | 26   | 0                    | 49                | 11                            | 22.5                                                           |
| 6                       | [1.37 , 1.59)          | 18   | 0                    | 26.9              | 5.64                          | 21                                                             |
| 7                       | [1.59 , 1.8)           | 8    | 0                    | 13.1              | 2.72                          | 20.7                                                           |

TABLE XX: The number of events for the data, the cosmic background, the CC1p signal, the beam related MC background and the fraction of the latter over the CC1p signal as a function of  $Q^2$ , after normalizing to  $4.59 \times 10^{19}$  POT.

| $Q^2$<br>Bin Number | $Q^2$<br>Bin Range | Data | Cosmic<br>Background | CC1p<br>MC Signal | Beam Related<br>MC Background | $\frac{\text{Beam Related MC BG}}{\text{CC1p MC Signal}} (\%)$ |
|---------------------|--------------------|------|----------------------|-------------------|-------------------------------|----------------------------------------------------------------|
| 1                   | [0 , 0.171)        | 93   | 3.53                 | 142               | 48                            | 33.9                                                           |
| 2                   | [0.171 , 0.343)    | 147  | 6.36                 | 170               | 39.6                          | 23.2                                                           |
| 3                   | [0.343 , 0.514)    | 98   | 3.53                 | 92.2              | 19.1                          | 20.7                                                           |
| 4                   | [0.514 , 0.686)    | 46   | 0                    | 43.6              | 8.46                          | 19.4                                                           |
| 5                   | [0.686 , 0.857)    | 20   | 2.12                 | 17.3              | 4.15                          | 24                                                             |
| 6                   | [0.857 , 1.03)     | 7    | 0                    | 8.05              | 1.54                          | 19.1                                                           |
| 7                   | [1.03 , 1.2)       | 1    | 0                    | 3.54              | 0.667                         | 18.8                                                           |

### INTERACTION BREAKDOWN

This section shows the interaction breakdown of the MC sample for one of the kinematic variables of interest, namely  $\cos\theta_\mu$ , as shown in figure 9, illustrating the dominance of QE interactions after the application of our selection cuts, while table XXI shows the relevant interaction breakdown for the entire sample of selected MC events. The same nominal MC sample is also used to compute the purity. Figures 10–11 and tables XXII–XXIII show the same breakdown for the CC1p signal and non-CC1p background parts of the MC sample respectively.

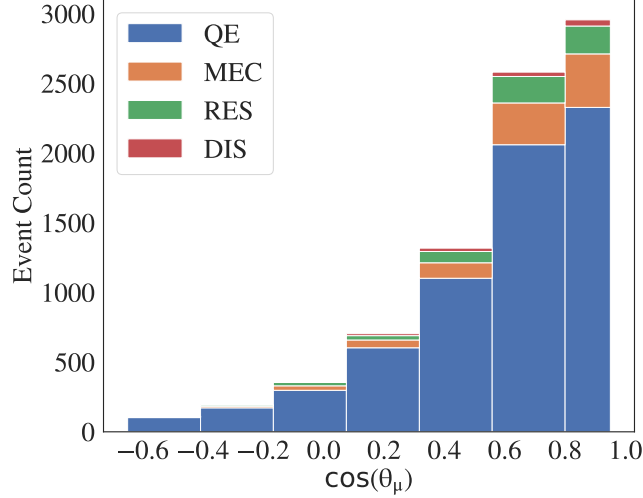

FIG. 9. Interaction breakdown of the  $\cos\theta_\mu$  plot illustrating the dominance of QE interactions after the application of our selection cuts in MC sample.

TABLE XXI: Interaction breakdown in the MC sample after the application of our selection cuts.

| Interaction<br>Mode | Fractional<br>Contribution (%) |
|---------------------|--------------------------------|
| QE                  | 81.1                           |
| MEC                 | 10.9                           |
| RES                 | 6.6                            |
| DIS                 | 1.4                            |

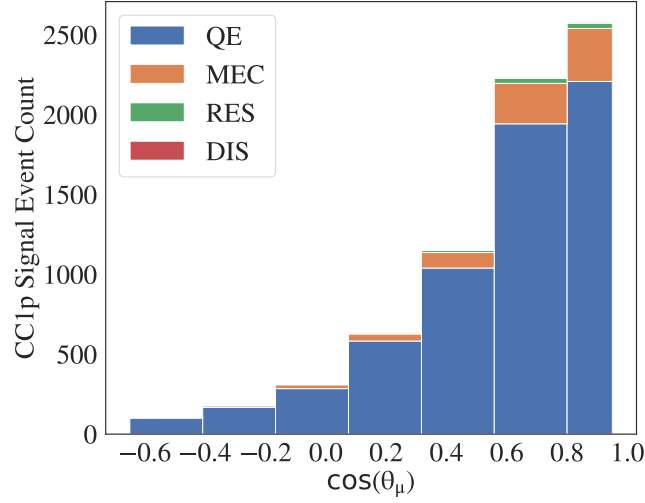

FIG. 10. Interaction breakdown of the  $\cos\theta_\mu$  plot illustrating the dominance of QE interactions after the application of our selection cuts for the CC1p signal part of the MC sample.

TABLE XXII: Interaction breakdown for the CC1p signal after the application of our selection cuts.

| Interaction Mode | Fractional Contribution (%) |
|------------------|-----------------------------|
| QE               | 87.9                        |
| MEC              | 10.6                        |
| RES              | 1.2                         |
| DIS              | 0.2                         |

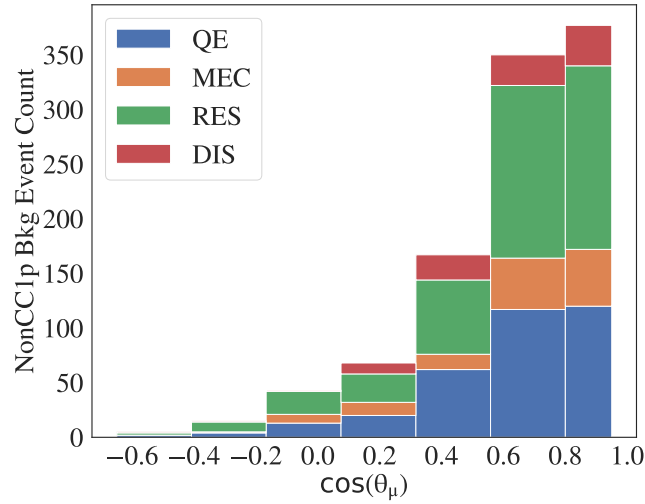

FIG. 11. Interaction breakdown of the  $\cos\theta_\mu$  plot illustrating the dominance of RES interactions after the application of our selection cuts for the non-CC1p background part of the MC sample.

TABLE XXIII: Interaction breakdown for the non-CC1p background after the application of our selection cuts.

| Interaction Mode | Fractional Contribution (%) |
|------------------|-----------------------------|
| QE               | 33.0                        |
| MEC              | 13.1                        |
| RES              | 44.1                        |
| DIS              | 9.9                         |

## DETECTOR SYSTEMATIC UNCERTAINTIES

In order to assess the detector systematic uncertainties, several samples are generated, where one detector parameter is varied at a time, and the same neutrino events are generated on top of the same cosmic background. Each of the following detector parameters are varied by  $1\sigma$ : longitudinal diffusion value, light yield outside the TPC, transverse diffusion, electron lifetime, recombination model and space charge map. The electronic response variation uses simulated neutrino events on top of a simulated cosmic background with **CORSIKA** [1]. The cross section is extracted using each one of those samples instead of the nominal simulation, where the relevant efficiencies, beam related background and data driven correction are rederived using the same procedures described in the paper. The uncertainty for each sample is obtained as the difference between the nominal cross section and the variation sample.

In order to address the deficit in the central  $\phi$  bin due to the missing dynamically induced charge effects, we apply a data driven correction, as described in the paper. We estimate the uncertainty due to this procedure by producing a dedicated dynamically induced charge variation sample and by treating the sample as data. The difference between the cross section extracted using this variation as data and the nominal MC cross section results is assigned to be the uncertainty due to our data driven correction.

The uncertainties discussed above are added in quadrature to obtain the total detector systematic uncertainty.

## EFFECTIVE EFFECIENCY

We extract the kinematic cross sections of interest as a function of the true variables by dividing by the effective efficiency  $\epsilon$ , which accounts both for the detection efficiency and the bin migration effects due to the finite detector resolution. For each bin  $n$ ,  $\epsilon_n$  is defined as the ratio of the number of reconstructed CC1p0 $\pi$  events to the number of generated true CC1p0 $\pi$  events, i.e.,

$$\begin{aligned}
\epsilon_n &= \frac{N_{\text{reconstructed in bin } n}^{\text{true CC1p0}\pi} (\text{generated in any bin})}{N_{\text{generated in bin } n}^{\text{true CC1p0}\pi}} \\
&= \frac{N_{\text{reconstructed in any bin}}^{\text{true CC1p0}\pi} (\text{generated in bin } n)}{N_{\text{generated in bin } n}^{\text{true CC1p0}\pi}} \\
&+ \frac{\sum_{j=1}^{N_{\text{bins}}} N_{\text{reconstructed in bin } n}^{\text{true CC1p0}\pi} (\text{generated in bin } j \neq n)}{N_{\text{generated in bin } n}^{\text{true CC1p0}\pi}} \\
&- \frac{\sum_{k=1}^{N_{\text{bins}}} N_{\text{reconstructed in bin } k \neq n}^{\text{true CC1p0}\pi} (\text{generated in bin } n)}{N_{\text{generated in bin } n}^{\text{true CC1p0}\pi}}
\end{aligned} \tag{1}$$

The generated events are restricted to the same phase-space limits as the reconstructed ones. The first component of equation 1, is the standard efficiency for events generated and reconstructed in the same bin. The second and third components account for bin-migration (in and out). Figure 12 shows the extracted efficiencies after the application of our selection cuts.

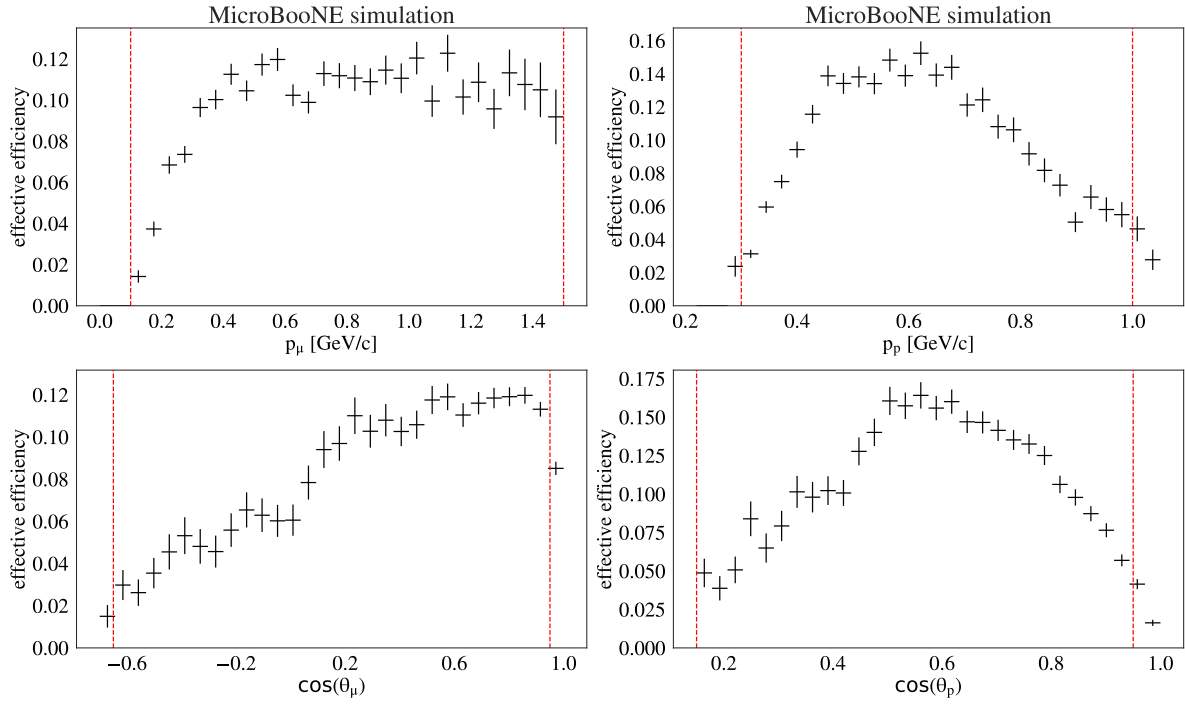

FIG. 12. Extracted efficiencies using the MicroBooNE MC after the application of our selection cuts.

## RESULTS WITHOUT BIN MIGRATION EFFECTS

In this section, we include the extracted cross-section without bin migration effects and we compare them to our nominal results shown in Figures 13–15. Tables XXIV–XXVII show the fractional correction due to bin migration effects for each one of the kinematic variables. This exercise shows that bin migration effects on this measurement are small and within the assessed uncertainties.

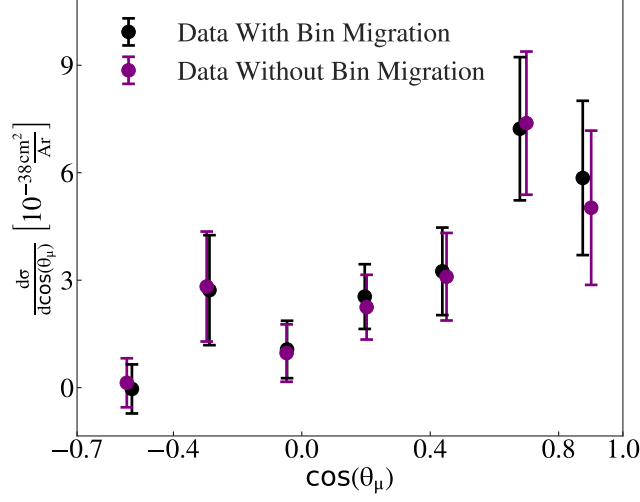

FIG. 13. The flux integrated single differential CC1p0 $\pi$  cross sections as a function of the cosine of the measured muon scattering angle with and without bin migration effects. Inner and outer error bars show the statistical and total (statistical and systematic) uncertainty at the  $1\sigma$ , or 68%, confidence level.

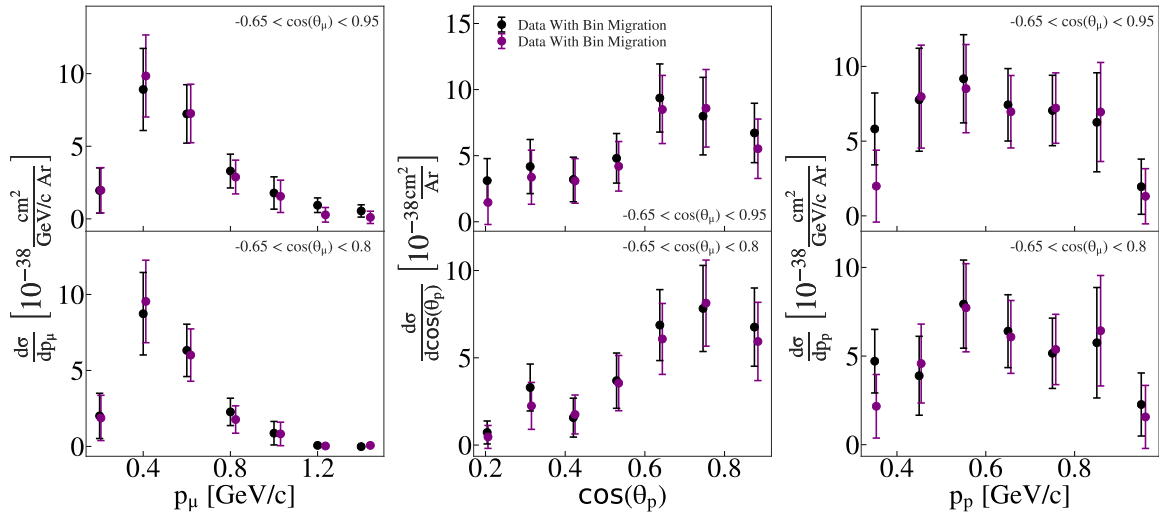

FIG. 14. As Fig. 13, but for the differential cross sections as a function of measured muon momentum (left) and measured proton scattering angle (middle) and momentum (right) with and without bin migration effects. Cross sections are shown for the full measured phase-space (top) and for events with  $\cos(\theta_\mu) < 0.8$  (bottom).

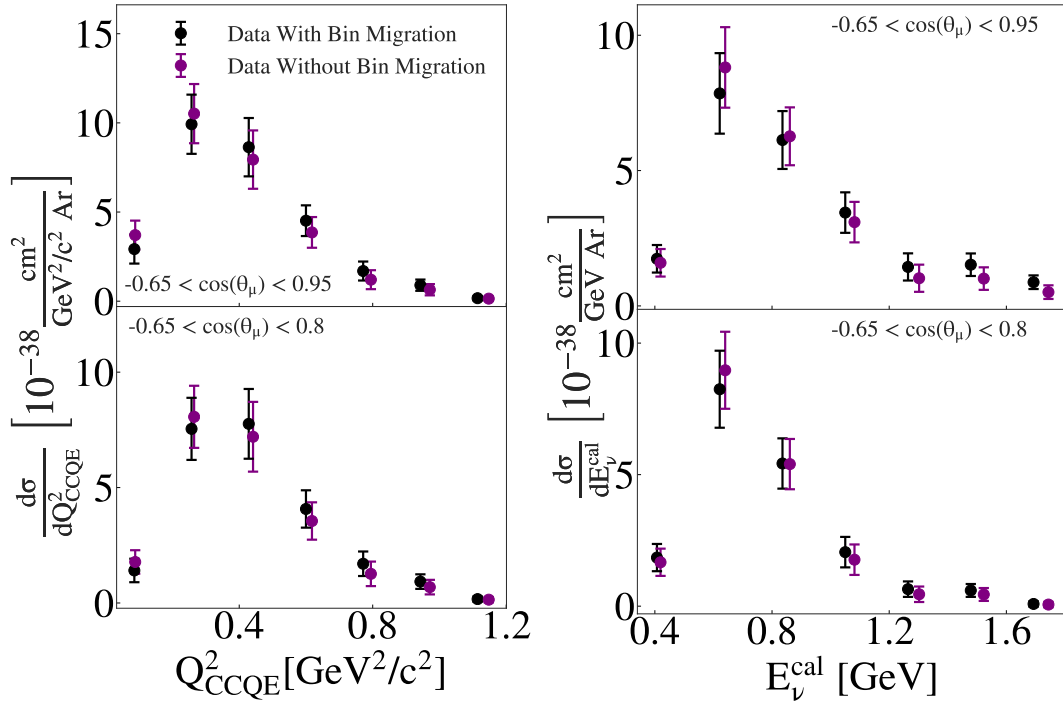

FIG. 15. The flux integrated single differential CC1p0 $\pi$  cross sections as a function of  $Q_{CCQE}^2 = (E_\nu^{cal} - E_\mu)^2 - (\vec{p}_\nu - \vec{p}_\mu)^2$  and  $E_\nu^{cal} = E_\mu + T_p + BE$ , where  $BE = 40$  MeV and  $\vec{p}_\nu = (0, 0, E_\nu^{cal})$ , without bin migration effects. Inner and outer error bars show the statistical and total (statistical and systematic) uncertainty at the  $1\sigma$ , or 68%, confidence level.

TABLE XXIV: The extracted data cross sections with and without bin migration effects and the fractional bin migration correction for the  $\cos(\theta_\mu)$  results.

| $\cos(\theta_\mu)$<br>Bin Number | $\cos(\theta_\mu)$<br>Bin Range | Data Cross Section<br>With Bin Migration | Data Cross Section<br>Without Bin Migration | Data Cross Section Error<br>Without Bin Migration |
|----------------------------------|---------------------------------|------------------------------------------|---------------------------------------------|---------------------------------------------------|
| 1                                | $[-0.65, -0.41)$                | -0.04                                    | 0.14                                        | 0.72                                              |
| 2                                | $[-0.41, -0.17)$                | 2.72                                     | 2.82                                        | 1.36                                              |
| 3                                | $[-0.17, 0.07)$                 | 1.07                                     | 0.96                                        | 0.56                                              |
| 4                                | $[0.07, 0.32)$                  | 2.54                                     | 2.25                                        | 0.66                                              |
| 5                                | $[0.32, 0.56)$                  | 3.25                                     | 3.1                                         | 1.09                                              |
| 6                                | $[0.56, 0.80)$                  | 7.23                                     | 7.38                                        | 1.87                                              |
| 7                                | $[0.80, 0.95)$                  | 5.85                                     | 5.02                                        | 1.7                                               |

TABLE XXV: The extracted data cross sections with and without bin migration effects and the fractional bin migration correction for the muon momentum results.

| $P_\mu$<br>Bin Number | $P_\mu$<br>Bin Range | Data Cross Section<br>With Bin Migration | Data Cross Section<br>Without Bin Migration | Data Cross Section Error<br>Without Bin Migration |
|-----------------------|----------------------|------------------------------------------|---------------------------------------------|---------------------------------------------------|
| 1                     | $[0.10, 0.30)$       | 1.95                                     | 1.97                                        | 1.34                                              |
| 2                     | $[0.30, 0.50)$       | 8.91                                     | 9.84                                        | 2.6                                               |
| 3                     | $[0.50, 0.70)$       | 7.23                                     | 7.26                                        | 1.83                                              |
| 4                     | $[0.70, 0.90)$       | 3.29                                     | 2.88                                        | 0.94                                              |
| 5                     | $[0.90, 1.10)$       | 1.78                                     | 1.55                                        | 0.98                                              |
| 6                     | $[1.10, 1.30)$       | 0.94                                     | 0.28                                        | 0.37                                              |
| 7                     | $[1.30, 1.50)$       | 0.54                                     | 0.1                                         | 0.32                                              |

TABLE XXVI: The extracted data cross sections with and without bin migration effects and the fractional bin migration correction for the  $\cos(\theta_p)$  results.

| $\cos(\theta_p)$<br>Bin Number | $\cos(\theta_p)$<br>Bin Range | Data Cross Section<br>With Bin Migration | Data Cross Section<br>Without Bin Migration | Data Cross Section Error<br>Without Bin Migration |
|--------------------------------|-------------------------------|------------------------------------------|---------------------------------------------|---------------------------------------------------|
| 1                              | [ 0.15 , 0.26 )               | 3.11                                     | 1.46                                        | 1.2                                               |
| 2                              | [ 0.26 , 0.37 )               | 4.18                                     | 3.37                                        | 1.71                                              |
| 3                              | [ 0.37 , 0.47 )               | 3.2                                      | 3.09                                        | 1.38                                              |
| 4                              | [ 0.47 , 0.58 )               | 4.8                                      | 4.2                                         | 1.61                                              |
| 5                              | [ 0.58 , 0.69 )               | 9.36                                     | 8.49                                        | 2.16                                              |
| 6                              | [ 0.69 , 0.80 )               | 7.99                                     | 8.59                                        | 2.52                                              |
| 7                              | [ 0.80 , 0.95 )               | 6.72                                     | 5.52                                        | 1.92                                              |

TABLE XXVII: The extracted data cross sections with and without bin migration effects and the fractional bin migration correction for the proton momentum results.

| $P_p$<br>Bin Number | $P_p$<br>Bin Range | Data Cross Section<br>With Bin Migration | Data Cross Section<br>Without Bin Migration | Data Cross Section Error<br>Without Bin Migration |
|---------------------|--------------------|------------------------------------------|---------------------------------------------|---------------------------------------------------|
| 1                   | [ 0.30 , 0.40 )    | 5.82                                     | 1.99                                        | 1.79                                              |
| 2                   | [ 0.40 , 0.50 )    | 7.77                                     | 7.98                                        | 3.23                                              |
| 3                   | [ 0.50 , 0.60 )    | 9.17                                     | 8.51                                        | 2.69                                              |
| 4                   | [ 0.60 , 0.70 )    | 7.43                                     | 6.97                                        | 2.12                                              |
| 5                   | [ 0.70 , 0.80 )    | 7.05                                     | 7.21                                        | 1.95                                              |
| 6                   | [ 0.80 , 0.90 )    | 6.26                                     | 6.95                                        | 2.88                                              |
| 7                   | [ 0.90 , 1.00 )    | 1.95                                     | 1.31                                        | 1.39                                              |

TABLE XXVIII: The extracted data cross sections with and without bin migration effects and the fractional bin migration correction for  $Q_{CCQE}^2$ .

| $Q_{CCQE}^2$<br>Bin Number | $Q_{CCQE}^2$<br>Bin Range | Data Cross Section<br>With Bin Migration | Data Cross Section<br>Without Bin Migration | Data Cross Section Error<br>Without Bin Migration |
|----------------------------|---------------------------|------------------------------------------|---------------------------------------------|---------------------------------------------------|
| 1                          | [ 0.00 , 0.17 )           | 2.92                                     | 3.71                                        | 0.88                                              |
| 2                          | [ 0.17 , 0.34 )           | 9.92                                     | 10.52                                       | 1.65                                              |
| 3                          | [ 0.34 , 0.51 )           | 8.64                                     | 7.94                                        | 1.59                                              |
| 4                          | [ 0.51 , 0.69 )           | 4.51                                     | 3.86                                        | 0.82                                              |
| 5                          | [ 0.69 , 0.86 )           | 1.69                                     | 1.21                                        | 0.49                                              |
| 6                          | [ 0.86 , 1.03 )           | 0.9                                      | 0.64                                        | 0.36                                              |
| 7                          | [ 1.03 , 1.20 )           | 0.17                                     | 0.14                                        | 0.17                                              |

TABLE XXIX: The extracted data cross sections with and without bin migration effects and the fractional bin migration correction for  $E_\nu^{cal}$ .

| $E_\nu^{cal}$<br>Bin Number | $E_\nu^{cal}$<br>Bin Range | Data Cross Section<br>With Bin Migration | Data Cross Section<br>Without Bin Migration | Data Cross Section Error<br>Without Bin Migration |
|-----------------------------|----------------------------|------------------------------------------|---------------------------------------------|---------------------------------------------------|
| 1                           | [ 0.30 , 0.51 )            | 1.74                                     | 1.59                                        | 0.53                                              |
| 2                           | [ 0.51 , 0.73 )            | 7.85                                     | 8.81                                        | 1.49                                              |
| 3                           | [ 0.73 , 0.94 )            | 6.13                                     | 6.27                                        | 1.09                                              |
| 4                           | [ 0.94 , 1.16 )            | 3.45                                     | 3.1                                         | 0.69                                              |
| 5                           | [ 1.16 , 1.37 )            | 1.44                                     | 1.02                                        | 0.42                                              |
| 6                           | [ 1.37 , 1.59 )            | 1.52                                     | 1.01                                        | 0.33                                              |
| 7                           | [ 1.59 , 1.80 )            | 0.88                                     | 0.51                                        | 0.21                                              |

## EVENT GENERATORS

This section includes a brief discussion of the underlying model configuration used in the different event generator predictions included in this analysis.

- **GENIE Nominal:** GENIE v2.12.2 [2, 3] with the Bodek-Ritchie Fermi Gas model, the Llewellyn-Smith CCQE scattering prescription [4], and the empirical meson exchange current (MEC) model [5], a Rein-Sehgal resonance (RES) and coherent scattering (COH) model [6], and a data driven final state interaction (FSI) model denoted as “hA” [7].
- **GENIE v3.0.6:** Using the Local Fermi Gas model [8], the Nieves CCQE scattering prescription [9] which includes Coulomb corrections for the outgoing muon [10] and Random Phase Approximation correction [11], the Nieves MEC model [12], the KLN-BS RES [13–16] and BS COH [17] scattering models, and the hA2018 FSI model [18].
- **NuWro 19.02.1** [19]: Using the Local Fermi Gas model [8], the Llewellyn-Smith CCQE scattering prescription [4], the Transverse Enhancement model for two-body currents [20], the Adler-Rarita-Schwinger formalism to calculate the  $\Delta$  resonance explicitly [21], the BS COH [17] scattering model and an intranuclear cascade model for FSI.
- **NEUT v5.4.0** [22]: Using the Local Fermi Gas model [8], the Nieves CCQE scattering prescription [9], the Nieves MEC model [12], the BS RES [13–16] and Rein-Sehgal COH [6] scattering models, and FSI with Oset medium correction for pions [2, 3].
- **GiBUU 2019:** Using somewhat similar models, but unlike in other generators, those are implemented in a coherent way, by solving the Boltzmann Uehling Uhlenbeck transport equation [23]. The models include: Local Fermi Gas model [8], standard CCQE expression [24], empirical MEC model and a dedicated spin dependent resonances amplitude calculation following the MAID analysis [25]. The DIS model is as in PYTHIA [26] and the FSI treatment is different as the hadrons propagate through the residual nucleus in a nuclear potential which is consistent with the initial state.

The agreement between the “nominal” GENIE calculation and the MC prediction constitutes a closure test for our analysis.

## COMPARISONS TO GENIE VARIATIONS

Apart from the comparisons to the different event generators, we further include the predictions from two more GENIE variation models:

- hA2015: GENIE v2.12.2 with the Bodek-Ritchie Fermi Gas model, a more recent “hA2015” FSI model with Oset medium correction for pions [2, 3].
- Alternative: GENIE v2.12.10 with the Local Fermi Gas model [8], the Nieves CCQE scattering prescription [9], the Nieves MEC model [12], the KLN-BS RES [13–16] and BS COH [17] scattering models, and the hA2015 FSI model.

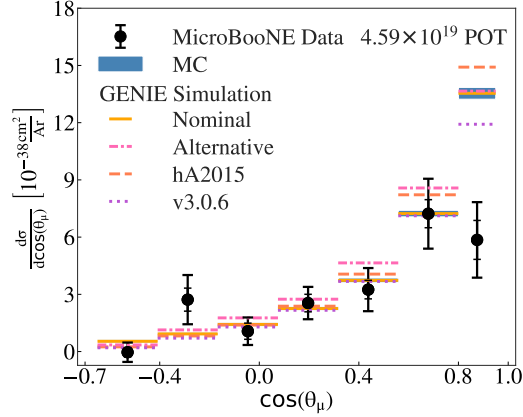

FIG. 16. The flux integrated single differential CC1p0 $\pi$  cross sections as a function of the cosine of the measured muon scattering angle. Inner and outer error bars show the statistical and total (statistical and systematic) uncertainty at the  $1\sigma$ , or 68%, confidence level. Colored lines show the results of theoretical absolute cross section calculations using different variations of the GENIE event generator (without passing through a detector simulation). The blue band shows the extracted cross section obtained from analyzing MC events propagated through our full detector simulation. The width of the band denotes the simulation statistical uncertainty.

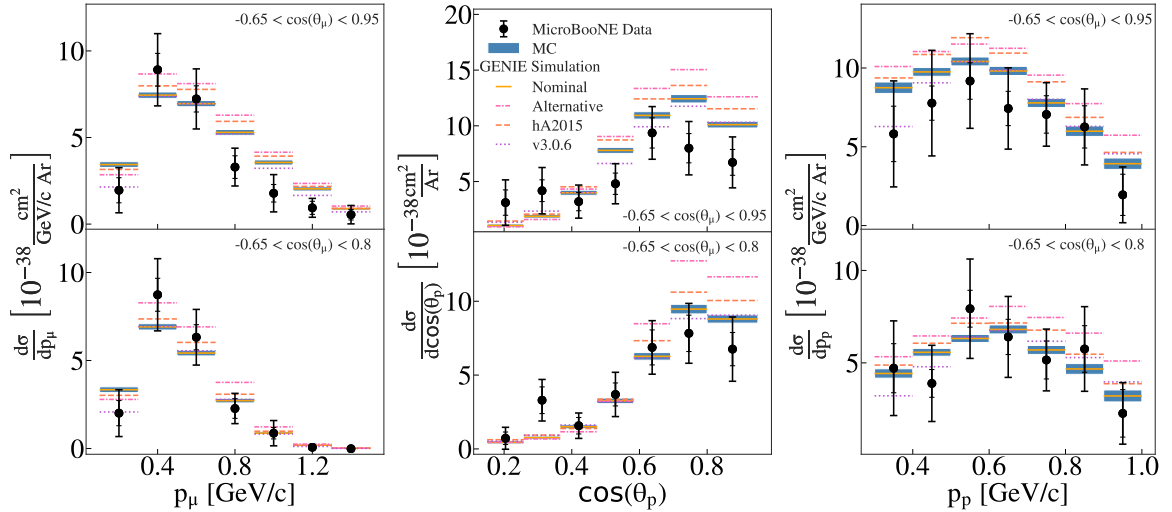

FIG. 17. As Fig. 16, but for the differential cross sections as a function of measured muon momentum (left) and measured proton scattering angle (middle) and momentum (right). Cross sections are shown for the full measured phase-space (top) and for events with  $\cos(\theta_\mu) < 0.8$  (bottom).

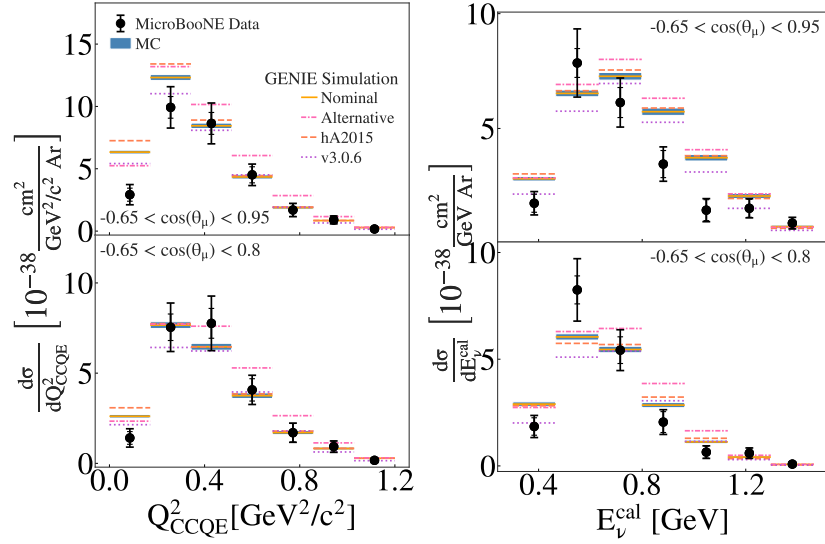

FIG. 18. The flux integrated single differential CC1p0 $\pi$  cross sections as a function of  $Q_{CCQE}^2 = (E_\nu^{cal} - E_\mu)^2 - (\vec{p}_\nu - \vec{p}_\mu)^2$  and  $E_\nu^{cal} = E_\mu + T_p + BE$ , where  $BE = 40$  MeV and  $\vec{p}_\nu = (0, 0, E_\nu^{cal})$ . Inner and outer error bars show the statistical and total (statistical and systematic) uncertainty at the  $1\sigma$ , or 68%, confidence level. Colored lines show the results of theoretical absolute cross section calculations using variations of the GENIE event generator (without passing through a detector simulation). The blue band shows the extracted cross section obtained from analyzing MC events passed through our full detector simulation.

### $\chi^2$ COMPARISONS

Tables XXX–XXXI show the extracted  $\chi^2/\text{d.o.f}$  for each one of the event generator simulation predictions, while table XXXVII shows the extracted  $\chi^2/\text{d.o.f}$  for the nominal MC sample used in this analysis, where the degrees of freedom are equal to the number of bins used in the cross section extraction as a function of each kinematic variable.

TABLE XXX: Extracted  $\chi^2/\text{d.o.f}$  for the data–nominal GENIE simulation comparison using both the full available phase space as well as the limited one with  $\cos(\theta_\mu) < 0.8$ .

| Kinematic Variable | $-0.65 < \cos(\theta_\mu) < 0.95$ | $-0.65 < \cos(\theta_\mu) < 0.8$ |
|--------------------|-----------------------------------|----------------------------------|
| $P_\mu$            | 14.2/7                            | 8.4/7                            |
| $\cos(\theta_\mu)$ | 33.8/7                            | 7.3/6                            |
| $P_p$              | 2.8/7                             | 5.1/7                            |
| $\cos(\theta_p)$   | 12.4/7                            | 9.2/7                            |

TABLE XXXI: Extracted  $\chi^2/\text{d.o.f}$  for the data–v3.0.6 GENIE simulation comparison using both the full available phase space as well as the limited one with  $\cos(\theta_\mu) < 0.8$ .

| Kinematic Variable | $-0.65 < \cos(\theta_\mu) < 0.95$ | $-0.65 < \cos(\theta_\mu) < 0.8$ |
|--------------------|-----------------------------------|----------------------------------|
| $P_\mu$            | 7.6/7                             | 4.6/7                            |
| $\cos(\theta_\mu)$ | 19.6/7                            | 5.1/6                            |
| $P_p$              | 1.8/7                             | 4.8/7                            |
| $\cos(\theta_p)$   | 5.6/7                             | 6.9/7                            |

TABLE XXXII: Extracted  $\chi^2/\text{d.o.f}$  for the data–NuWro simulation comparison using both the full available phase space as well as the limited one with  $\cos(\theta_\mu) < 0.8$ .

| Kinematic Variable | $-0.65 < \cos(\theta_\mu) < 0.95$ | $-0.65 < \cos(\theta_\mu) < 0.8$ |
|--------------------|-----------------------------------|----------------------------------|
| $P_\mu$            | 13.4/7                            | 5.3/7                            |
| $\cos(\theta_\mu)$ | 41.0/7                            | 7.2/6                            |
| $P_p$              | 7.7/7                             | 7.0/7                            |
| $\cos(\theta_p)$   | 14.6/7                            | 10.4/7                           |

TABLE XXXIII: Extracted  $\chi^2/\text{d.o.f}$  for the data–NEUT simulation comparison using both the full available phase space as well as the limited one with  $\cos(\theta_\mu) < 0.8$ .

| Kinematic Variable | $-0.65 < \cos(\theta_\mu) < 0.95$ | $-0.65 < \cos(\theta_\mu) < 0.8$ |
|--------------------|-----------------------------------|----------------------------------|
| $P_\mu$            | 16.8/7                            | 5.7/7                            |
| $\cos(\theta_\mu)$ | 38.9/7                            | 7.2/6                            |
| $P_p$              | 7.5/7                             | 11.7/7                           |
| $\cos(\theta_p)$   | 15.3/7                            | 7.6/7                            |

TABLE XXXIV: Extracted  $\chi^2/\text{d.o.f}$  for the data–GiBUU simulation comparison using both the full available phase space as well as the limited one with  $\cos(\theta_\mu) < 0.8$ .

| Kinematic Variable | $-0.65 < \cos(\theta_\mu) < 0.95$ | $-0.65 < \cos(\theta_\mu) < 0.8$ |
|--------------------|-----------------------------------|----------------------------------|
| $P_\mu$            | 23.9/7                            | 11.2/7                           |
| $\cos(\theta_\mu)$ | 35.8/7                            | 9.7/6                            |
| $P_p$              | 7.8/7                             | 7.2/7                            |
| $\cos(\theta_p)$   | 14.7/7                            | 11.9/7                           |

TABLE XXXV: Extracted  $\chi^2/\text{d.o.f}$  for the data–hA2015 GENIE simulation comparison using both the full available phase space as well as the limited one with  $\cos(\theta_\mu) < 0.8$ .

| Kinematic Variable | $-0.65 < \cos(\theta_\mu) < 0.95$ | $-0.65 < \cos(\theta_\mu) < 0.8$ |
|--------------------|-----------------------------------|----------------------------------|
| $P_\mu$            | 12.2/7                            | 7.5/7                            |
| $\cos(\theta_\mu)$ | 30.7/7                            | 4.6/6                            |
| $P_p$              | 3.0/7                             | 5.4/7                            |
| $\cos(\theta_p)$   | 10.5/7                            | 7.9/7                            |

TABLE XXXVI: Extracted  $\chi^2/\text{d.o.f}$  for the data–Alternative GENIE simulation comparison using both the full available phase space as well as the limited one with  $\cos(\theta_\mu) < 0.8$ .

| Kinematic Variable | $-0.65 < \cos(\theta_\mu) < 0.95$ | $-0.65 < \cos(\theta_\mu) < 0.8$ |
|--------------------|-----------------------------------|----------------------------------|
| $P_\mu$            | 12.8/7                            | 6.7/7                            |
| $\cos(\theta_\mu)$ | 20.8/7                            | 6.1/6                            |
| $P_p$              | 3.4/7                             | 5.8/7                            |
| $\cos(\theta_p)$   | 14.2/7                            | 15.2/7                           |

TABLE XXXVII: Extracted  $\chi^2/\text{d.o.f}$  for the data–Overlay MC GENIE simulation comparison using both the full available phase space as well as the limited one with  $\cos(\theta_\mu) < 0.8$ .

| Kinematic Variable | $-0.65 < \cos(\theta_\mu) < 0.95$ | $-0.65 < \cos(\theta_\mu) < 0.8$ |
|--------------------|-----------------------------------|----------------------------------|
| $P_\mu$            | 14.2/7                            | 8.4/7                            |
| $\cos(\theta_\mu)$ | 33.8/7                            | 7.3/6                            |
| $P_p$              | 2.8/7                             | 5.1/7                            |
| $\cos(\theta_p)$   | 12.4/7                            | 9.2/7                            |

### VERTEX Z DISTRIBUTION

The measured  $z$ -vertex distribution, after the beam related MC background has been subtracted, does not show an excess at low- $z$ , which indicates that background events from interactions upstream of the detector are not accidentally entering our selection, which would show up as a small- $z$  enhancement in our vertex distribution. The deficit at  $z = 700$  cm is due to dead wires in our detector and its effect has been incorporated in our simulation.

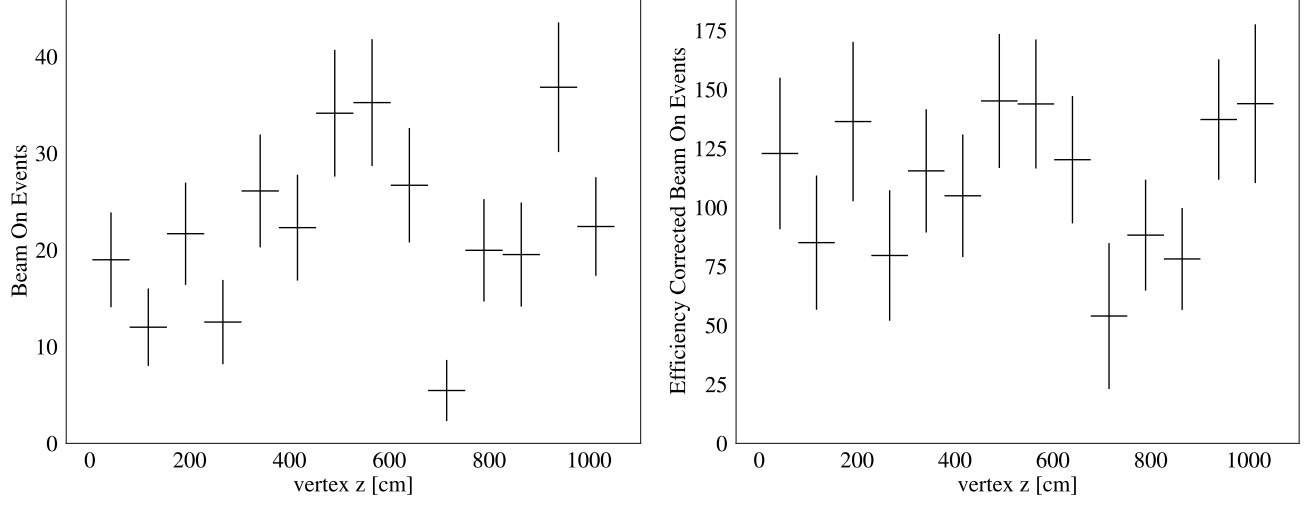

FIG. 19. Vertex  $z$  distribution for the measured events, after the beam related MC background has been subtracted, before (left) and after (right) detection efficiency corrections. No small- $z$  enhancement is observed and, with efficiency corrections, the measured distribution is consistent with that of a uniform neutrino interaction vertex.

- 
- [1] D. Heck, J. Knapp, J. Capdevielle, G. Schatz, and T. Thouw, (1998).
  - [2] C. Andreopoulos *et al.*, *Nucl. Instrum. Meth. A* , 87.
  - [3] C. Andreopoulos *et al.*, (2015), [arXiv:1510.05494 \[hep-ph\]](#).
  - [4] C. Llewellyn Smith, *Phys. Rept.* **3**, 261 (1972).
  - [5] T. Katori, *AIP Conf. Proc.* **1663**, 030001 (2015).
  - [6] D. Rein and L. Sehgal, *Annals Phys.* **133**, 79 (1981).
  - [7] S. Mashnik *et al.*, *J. Phys. Conf. Ser.* **41**, 340 (2006).
  - [8] R. Carrasco and E. Oset, *Nucl. Phys. A* **536**, 445 (1992).
  - [9] J. Nieves, F. Sanchez, I. Ruiz Simo, and M. Vicente Vacas, *Phys. Rev. D* **85**, 113008 (2012).
  - [10] J. Engel, *Phys. Rev. C* **57**, 2004 (1998), [arXiv:nucl-th/9711045](#).
  - [11] J. Nieves, J. E. Amaro, and M. Valverde, *Phys. Rev. C* **70**, 055503 (2004).
  - [12] J. Schwehr, D. Cherdack, and R. Gran, (2016), [arXiv:1601.02038 \[hep-ph\]](#).
  - [13] J. A. Nowak (MiniBooNE Collaboration), *AIP Conf. Proc.* **1189**, 243 (2009).
  - [14] K. Kuzmin *et al.*, *Phys. Part. Nucl.* **35**, S133 (2004).
  - [15] C. Berger and L. Sehgal, *Phys. Rev. D* **76**, 113004 (2007).
  - [16] K. M. Graczyk and J. T. Sobczyk, *Phys. Rev. D* **77**, 053001 (2008), [Erratum: *Phys.Rev.D* 79, 079903 (2009)].
  - [17] C. Berger and L. Sehgal, *Phys. Rev. D* **79**, 053003 (2009).
  - [18] D. Ashery, I. Navon, G. Azuelos, H. Walter, H. Pfeiffer, and F. Schleputz, *Phys. Rev. C* **23**, 2173 (1981).
  - [19] T. Golan *et al.*, *Nucl.Phys.Proc.Suppl.* **499**, 229 (2012).
  - [20] A. Bodek *et al.*, *Eur. Phys. J. C* **71**, 1726 (2011).
  - [21] K. Graczyk *et al.*, *Phys. Rev. D* **80**, 093001 (2009).
  - [22] Y. Hayato, *Acta Phys. Polon.* **B40**, 2477 (2009).
  - [23] U. Mosel, *Phys. Rev. G* (2019), [10.1088/1361-6471/ab3830](#), [arXiv:1361-6471 \[hep-ex\]](#).
  - [24] T. Leitner, L. Alvarez-Ruso, and U. Mosel, *Phys. Rev. C* **73**, 065502 (2006), [arXiv:nucl-th/0601103](#).
  - [25] U. Mosel, *J. Phys. G* **46**, 113001 (2019), [arXiv:1904.11506 \[hep-ex\]](#).
  - [26] T. Sjostrand, S. Mrenna, and P. Z. Skands, *JHEP* **05**, 026 (2006), [arXiv:hep-ph/0603175](#).
